# Supplementary material for: SemiCurv: Semi-Supervised Curvilinear Structure Segmentation
Source: arXiv:2205.08706 source file (2022-05-19)

RGB

Ground-Truth

Unet

CutMix

MT

SemiCurv

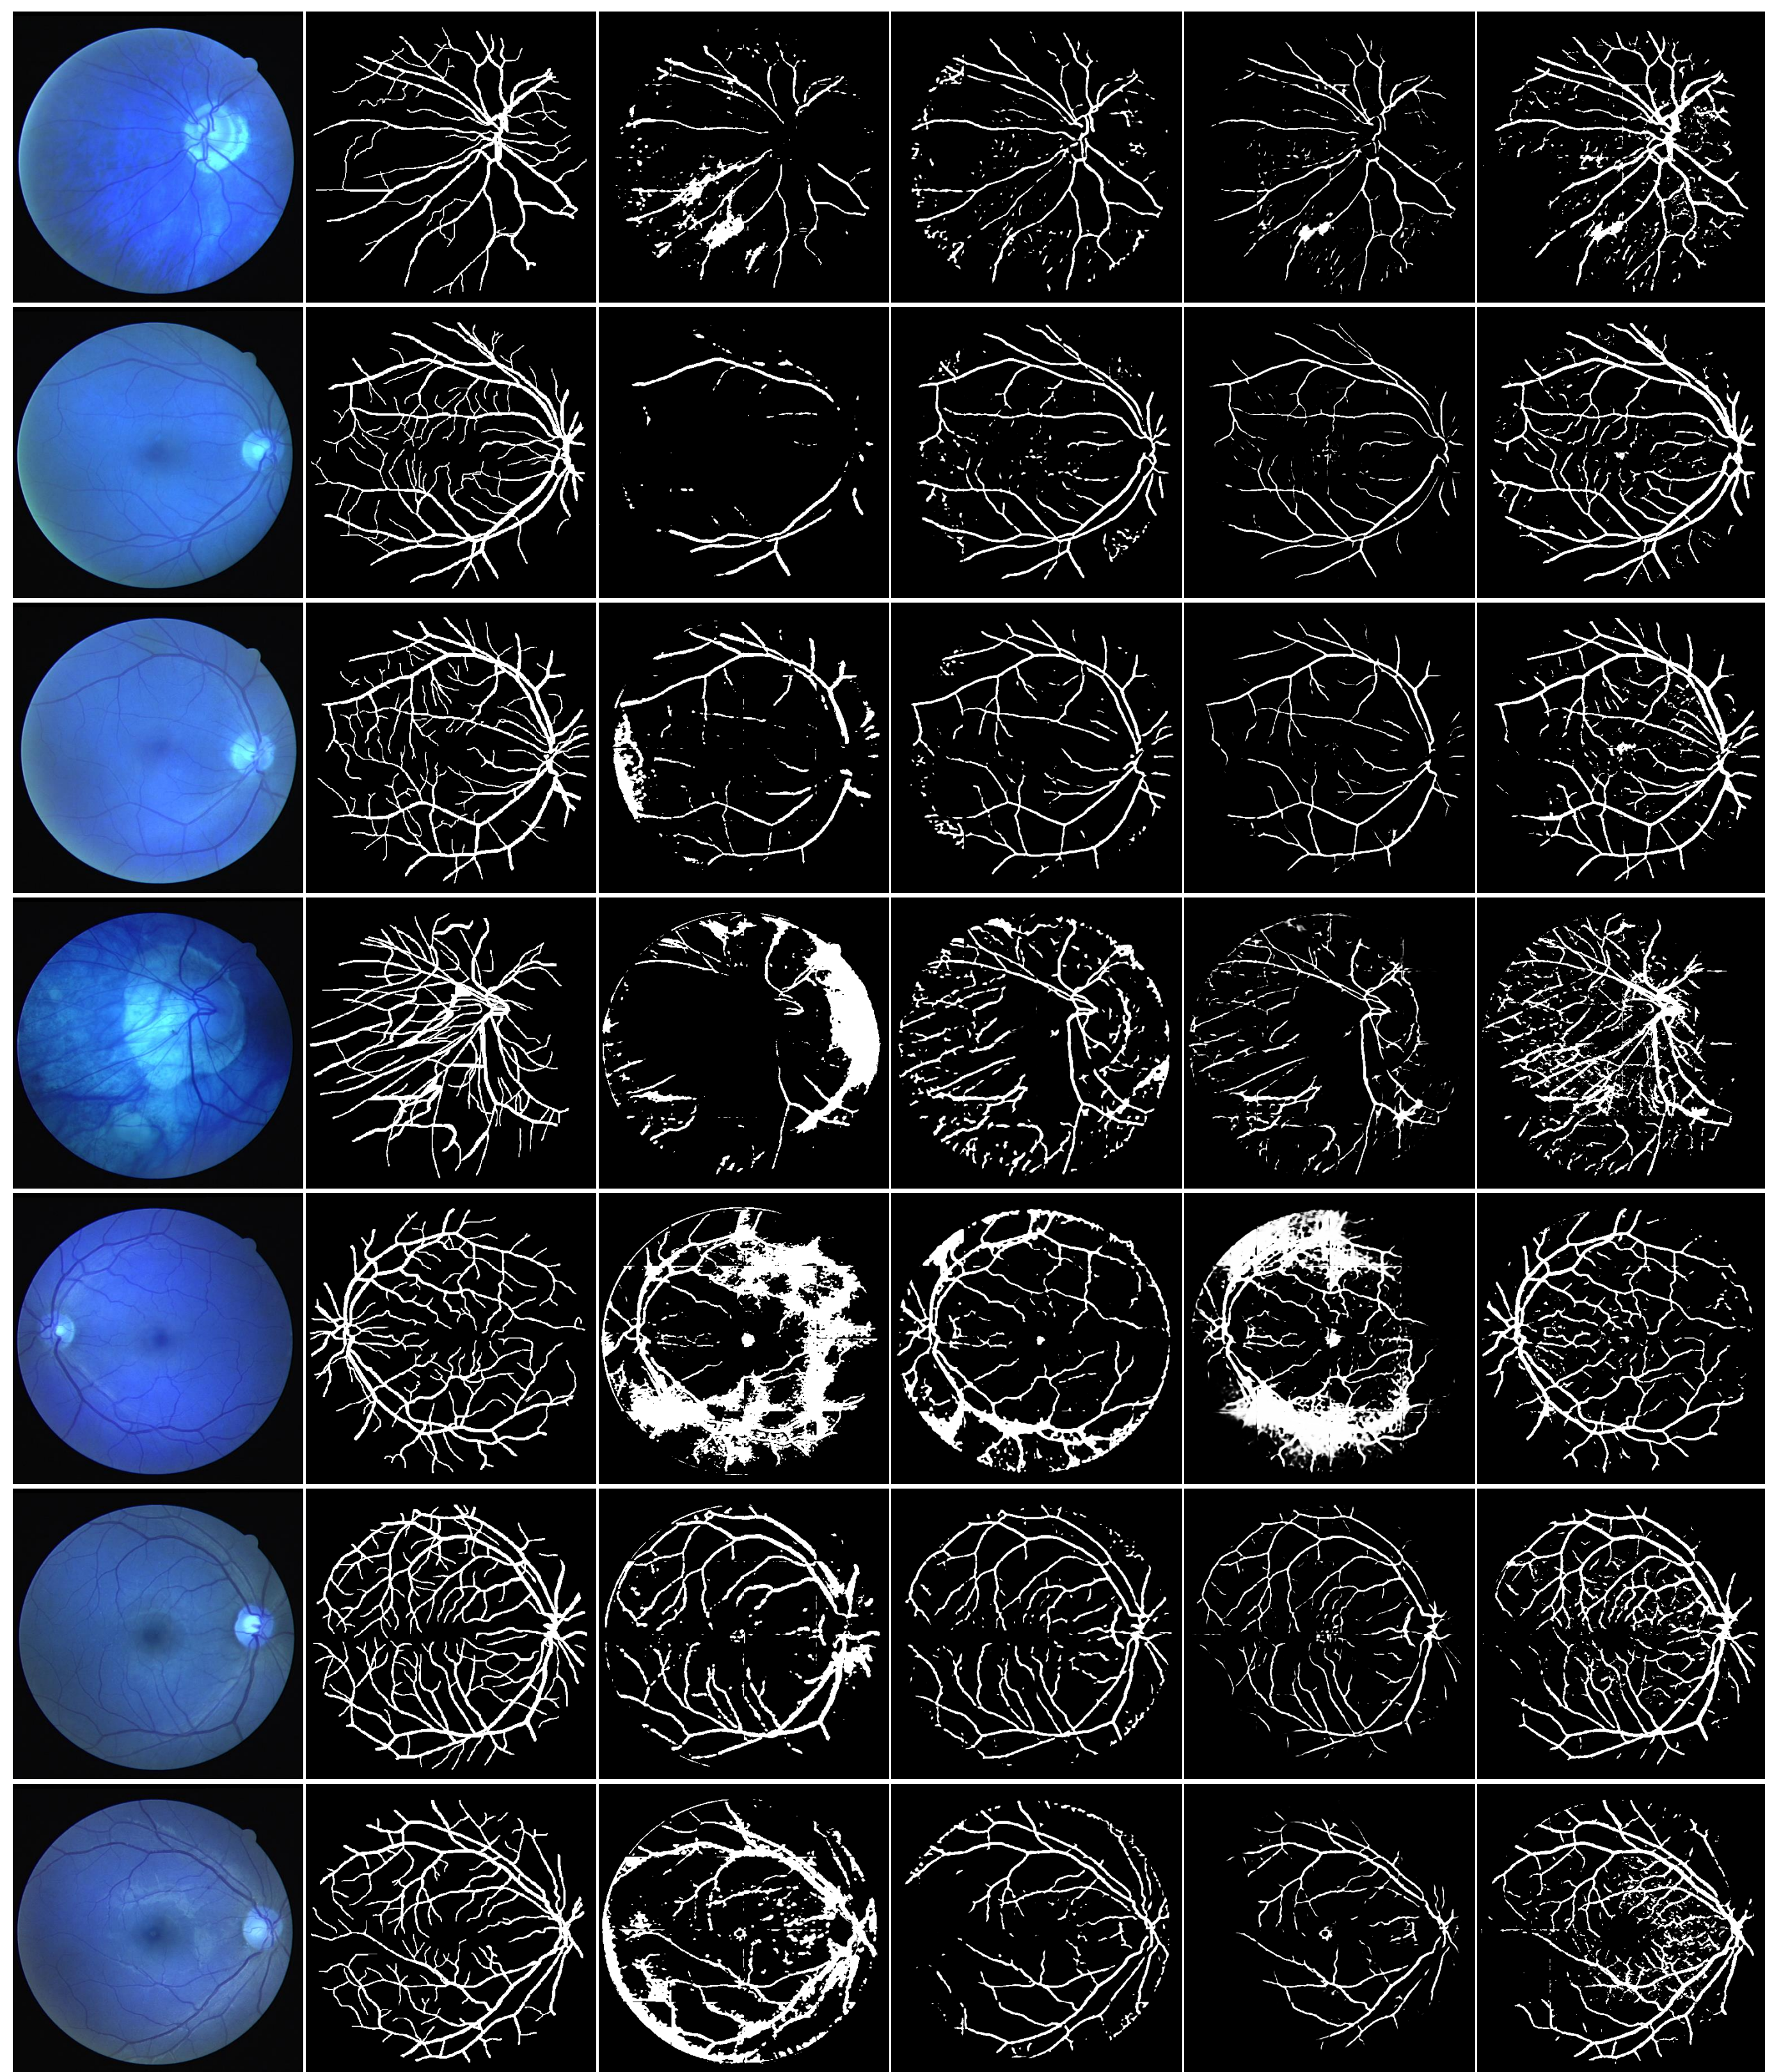



RGB

Ground-Truth

Unet

CutMix

MT

SemiCurv

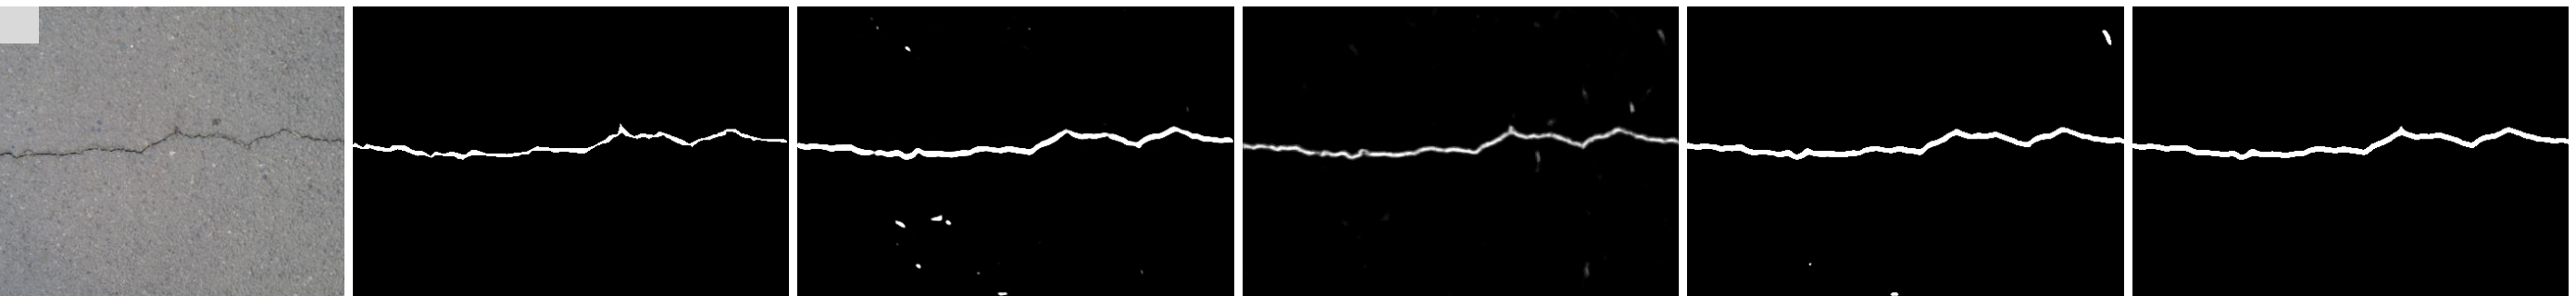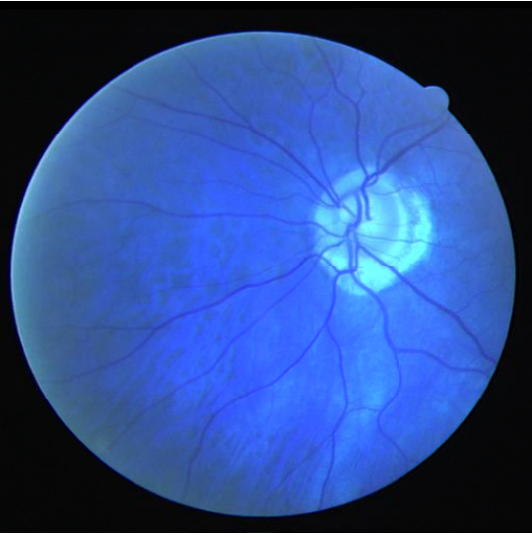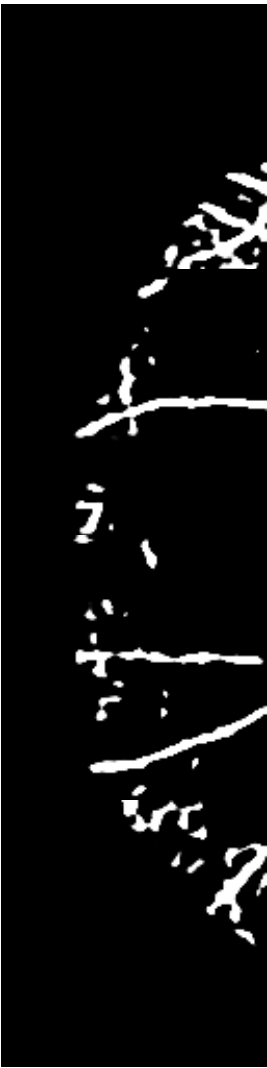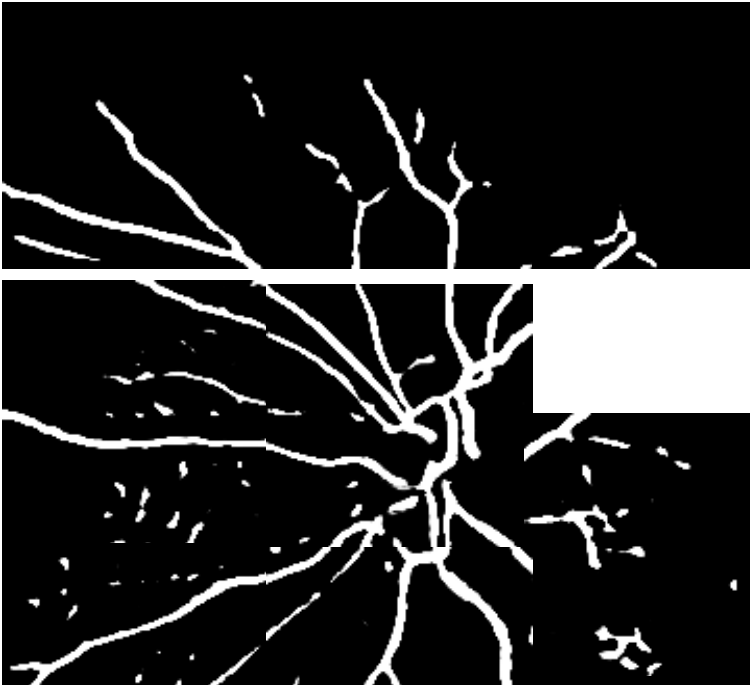

Supplement: Supplementary file 1 [file Supp_DRIVE128.pdf]
